# Supplementary material for: Reaction-diffusion equations with spatially distributed hysteresis
Source: arXiv:1205.3580 source file (2012-05-16)
Supplement: Supplementary file 1 [file appendix.tex]

\appendix

\section{Appendix: Proof of Lemma~$\ref{lab}$}\label{Appendix}

1. First, we let $\lambda = \gamma>0$. Note that $b(t)$ is a
nondecreasing function and
\begin{equation}\label{eqab1}
b(t_2) - b(t_1) \leq \max_{s \in [t_1, t_2]} a(s) - a(t_1), \quad
0 \leq t_1 \leq t_2 \leq T.
\end{equation}
 On the other hand, by the H\"older continuity of $a$,
\begin{equation}\label{eqab2}
|a(s_2) - a(s_1)| \le K |s_2-s_1|^{\gamma}, \quad s_1, s_2 \in [0,
T].
\end{equation}
where $$K=\sup\limits_{0\le t_1<t_2\le T}\dfrac{|a(t_2) -
a(t_1)|}{|t_2-t_1|^{\gamma}}.$$

Inequalities~\eqref{eqab1} and~\eqref{eqab2} imply that
$$
b(t_2) - b(t_1) \leq \max_{s \in [t_1, t_2]} a(s) - a(t_1) \le K
|t_2-t_1|^{\gamma}, \quad 0 \leq t_1 \leq t_2 \leq T,
$$
which proves part 1 of  Lemma~\ref{lab} for $\lambda=\gamma$.

Consider the case $\lambda = 0$. Fix $t_0 \in [0, T]$ and
$\varepsilon
> 0$. By the continuity of $a(t)$,  there exists $\delta > 0$ such
that
$$
|a(s) - a(t_0)| \le \varepsilon, \quad s \in [t_0 - \delta, t_0 +
\delta]
$$
(with obvious modification if $t_0=0$ of $T$). Hence, taking into
account~\eqref{eqab1}, we have
\begin{equation}\label{eqab3}
0 \leq b(t)- b(t_0) \leq \max_{s \in [t_0, t]} a(s) - a(t_0) \le
\varepsilon, \quad t \in [t_0, t_0 + \delta],
\end{equation}
if $t_0\ne T$ and
\begin{equation}\label{eqab4}
\begin{aligned}
&0 \leq b(t_0) - b(t) \leq \max_{s \in [t, t_0]} a(s) - a(t)
\\
&\qquad \leq \max_{s \in [t, t_0]} (a(s) - a(t_0)) + (a(t_0) -
a(t)) \leq 2 \varepsilon,\quad t\in [t_0-\delta,t_0],
\end{aligned}
\end{equation}
if $t_0\ne 0$. Inequalities~\eqref{eqab3} and~\eqref{eqab4} imply
the continuity of $b$.

2. Let us prove part 2 of  Lemma~\ref{lab}. Since $b_2(t)$ can be
represented as
$$
b_2(t)=\max\limits_{s\in[0,t]}(a_1(s)+[a_2(s)-a_1(s)]),
$$
we have
$$
b_2(t)\le b_1(t)+\|a_2-a_1\|_{C[0,T]},
$$
$$
b_2(t)\ge b_1(t)-\|a_2-a_1\|_{C[0,T]}.
$$
Combining these two inequalities, we complete the proof.
